# Supplementary material for: Robust 3D Gaussian Splatting for Novel View Synthesis in Presence of Distractors
Source: arXiv:2408.11697 source file (2024-08-21)
Supplement: Supplementary file 1 [file 7_appendix.tex]

\clearpage
\appendix

\begin{table*}[!ht]
    \centering
    \begin{tabularx}{\textwidth}{|>{\centering\arraybackslash}X|>{\centering\arraybackslash}X||>{\centering\arraybackslash}X|>{\centering\arraybackslash}X|>{\centering\arraybackslash}X|>{\centering\arraybackslash}X|>{\centering\arraybackslash}X|}
        \hline
        Scene&Metric&Gaussian Splatting&Robust NeRF&+Neural&+Segment.&+Both\\
        \hhline{|=|=#=|=|=|=|=|}
        &SSIM \(\uparrow\)&0.8401&0.8410&0.8416&0.8268&\textbf{0.8514}\\
        Statue&PSNR \(\uparrow\)&21.56&21.27&21.52&20.21&\textbf{22.21}\\
        &LPIPS \(\downarrow\)&0.1443&0.1374&0.1376&0.15926&\textbf{0.1214}\\
        \hline
        &SSIM&0.8957&0.8821&0.9129&0.9017&\textbf{0.9170}\\
        Yoda&PSNR&27.43&25.93&\textbf{30.62}&27.13&30.45\\
        &LPIPS&0.2001&0.2177&0.1746&0.1891&\textbf{0.15984}\\
        \hline
        &SSIM&0.8004&0.7952&0.8235&0.7794&\textbf{0.8240}\\
        And-bot&PSNR&23.63&22.71&24.40&21.51&\textbf{24.48}\\
        &LPIPS&0.15938&0.15922&\textbf{0.1308}&0.1778&0.1314\\
        \hline
        &SSIM&0.9385&0.9132&0.9481&0.8034&\textbf{0.9511}\\
        Crab&PSNR&30.92&26.46&33.46&21.62&\textbf{34.23}\\
        &LPIPS&0.1414&0.1919&0.1184&0.1765&\textbf{0.1151}\\
        \hhline{|=|=#=|=|=|=|=|}
        &SSIM&0.8687&0.8579&0.8815&0.8278&\textbf{0.8859}\\
        Mean&PSNR&25.89&24.09&27.50&22.62&\textbf{27.84}\\
        &LPIPS&0.15924&0.1773&0.1404&0.1740&\textbf{0.1341}\\
        \hline
    \end{tabularx}
    \caption{Quantitative results of tests with all ablations.}
    \label{tab:quant_results}
\end{table*}

\section{Further qualitative results}
\autoref{fig:qual_2} shows qualitative comparisons from all four test scenes. It reflects the results from \autoref{fig:example_comparison} where the +Both version achieves the best results.

\begin{figure*}[ht]
    \centering  
    \begin{subfigure}[t]{0.159\textwidth}
        \centering
        \frame{\includegraphics[width=\textwidth, keepaspectratio]{images/crab_2/baseline.png}}   
    \end{subfigure}    
    \hfill  
    \begin{subfigure}[t]{0.159\textwidth}
        \centering
        \frame{\includegraphics[width=\textwidth, keepaspectratio]{images/crab_2/robust.png}}   
    \end{subfigure}    
    \hfill  
    \begin{subfigure}[t]{0.159\textwidth}
        \centering
        \frame{\includegraphics[width=\textwidth, keepaspectratio]{images/crab_2/neural.png}}   
    \end{subfigure}    
    \hfill  
    \begin{subfigure}[t]{0.159\textwidth}
        \centering
        \frame{\includegraphics[width=\textwidth, keepaspectratio]{images/crab_2/seg.png}}   
    \end{subfigure}    
    \hfill  
    \begin{subfigure}[t]{0.159\textwidth}
        \centering
        \frame{\includegraphics[width=\textwidth, keepaspectratio]{images/crab_2/both.png}}   
    \end{subfigure}    
    \hfill
    \begin{subfigure}[t]{0.159\textwidth}
        \centering
        \frame{\includegraphics[width=\textwidth, keepaspectratio]{images/crab_2/gt.png}}   
    \end{subfigure}  
    \begin{subfigure}[t]{0.159\textwidth}
        \centering
        \frame{\includegraphics[width=\textwidth, keepaspectratio]{images/balloon/baseline.png}}   
    \end{subfigure}    
    \hfill  
    \begin{subfigure}[t]{0.159\textwidth}
        \centering
        \frame{\includegraphics[width=\textwidth, keepaspectratio]{images/balloon/robust.png}}   
    \end{subfigure}    
    \hfill  
    \begin{subfigure}[t]{0.159\textwidth}
        \centering
        \frame{\includegraphics[width=\textwidth, keepaspectratio]{images/balloon/neural.png}}   
    \end{subfigure}    
    \hfill  
    \begin{subfigure}[t]{0.159\textwidth}
        \centering
        \frame{\includegraphics[width=\textwidth, keepaspectratio]{images/balloon/seg.png}}   
    \end{subfigure}    
    \hfill  
    \begin{subfigure}[t]{0.159\textwidth}
        \centering
        \frame{\includegraphics[width=\textwidth, keepaspectratio]{images/balloon/both.png}}   
    \end{subfigure}    
    \hfill
    \begin{subfigure}[t]{0.159\textwidth}
        \centering
        \frame{\includegraphics[width=\textwidth, keepaspectratio]{images/balloon/gt.png}}   
    \end{subfigure}  
    \begin{subfigure}[t]{0.159\textwidth}
        \centering
        \frame{\includegraphics[width=\textwidth, keepaspectratio]{images/balloon_2/baseline.png}}   
    \end{subfigure}    
    \hfill  
    \begin{subfigure}[t]{0.159\textwidth}
        \centering
        \frame{\includegraphics[width=\textwidth, keepaspectratio]{images/balloon_2/robust.png}}   
    \end{subfigure}    
    \hfill  
    \begin{subfigure}[t]{0.159\textwidth}
        \centering
        \frame{\includegraphics[width=\textwidth, keepaspectratio]{images/balloon_2/neural.png}}   
    \end{subfigure}    
    \hfill  
    \begin{subfigure}[t]{0.159\textwidth}
        \centering
        \frame{\includegraphics[width=\textwidth, keepaspectratio]{images/balloon_2/seg.png}}   
    \end{subfigure}    
    \hfill  
    \begin{subfigure}[t]{0.159\textwidth}
        \centering
        \frame{\includegraphics[width=\textwidth, keepaspectratio]{images/balloon_2/both.png}}   
    \end{subfigure}    
    \hfill
    \begin{subfigure}[t]{0.159\textwidth}
        \centering
        \frame{\includegraphics[width=\textwidth, keepaspectratio]{images/balloon_2/gt.png}}   
    \end{subfigure}  
    \begin{subfigure}[t]{0.159\textwidth}
        \centering
        \frame{\includegraphics[width=\textwidth, keepaspectratio]{images/and_bot/baseline.png}}   
    \end{subfigure}    
    \hfill  
    \begin{subfigure}[t]{0.159\textwidth}
        \centering
        \frame{\includegraphics[width=\textwidth, keepaspectratio]{images/and_bot/robust.png}}   
    \end{subfigure}    
    \hfill  
    \begin{subfigure}[t]{0.159\textwidth}
        \centering
        \frame{\includegraphics[width=\textwidth, keepaspectratio]{images/and_bot/neural.png}}   
    \end{subfigure}    
    \hfill  
    \begin{subfigure}[t]{0.159\textwidth}
        \centering
        \frame{\includegraphics[width=\textwidth, keepaspectratio]{images/and_bot/seg.png}}   
    \end{subfigure}    
    \hfill  
    \begin{subfigure}[t]{0.159\textwidth}
        \centering
        \frame{\includegraphics[width=\textwidth, keepaspectratio]{images/and_bot/both.png}}   
    \end{subfigure}    
    \hfill
    \begin{subfigure}[t]{0.159\textwidth}
        \centering
        \frame{\includegraphics[width=\textwidth, keepaspectratio]{images/and_bot/gt.png}}   
    \end{subfigure}    
    \begin{subfigure}[t]{0.159\textwidth}
        \centering
        \frame{\includegraphics[width=\textwidth, keepaspectratio]{images/and_bot_2/baseline.png}}   
    \end{subfigure}    
    \hfill  
    \begin{subfigure}[t]{0.159\textwidth}
        \centering
        \frame{\includegraphics[width=\textwidth, keepaspectratio]{images/and_bot_2/robust.png}}   
    \end{subfigure}    
    \hfill  
    \begin{subfigure}[t]{0.159\textwidth}
        \centering
        \frame{\includegraphics[width=\textwidth, keepaspectratio]{images/and_bot_2/neural.png}}   
    \end{subfigure}    
    \hfill  
    \begin{subfigure}[t]{0.159\textwidth}
        \centering
        \frame{\includegraphics[width=\textwidth, keepaspectratio]{images/and_bot_2/seg.png}}   
    \end{subfigure}    
    \hfill  
    \begin{subfigure}[t]{0.159\textwidth}
        \centering
        \frame{\includegraphics[width=\textwidth, keepaspectratio]{images/and_bot_2/both.png}}   
    \end{subfigure}    
    \hfill
    \begin{subfigure}[t]{0.159\textwidth}
        \centering
        \frame{\includegraphics[width=\textwidth, keepaspectratio]{images/and_bot_2/gt.png}}   
    \end{subfigure} 
    \begin{subfigure}[t]{0.159\textwidth}
        \centering
        \frame{\includegraphics[width=\textwidth, keepaspectratio]{images/yoda/baseline.png}}   
    \end{subfigure}    
    \hfill  
    \begin{subfigure}[t]{0.159\textwidth}
        \centering
        \frame{\includegraphics[width=\textwidth, keepaspectratio]{images/yoda/robust.png}}   
    \end{subfigure}    
    \hfill  
    \begin{subfigure}[t]{0.159\textwidth}
        \centering
        \frame{\includegraphics[width=\textwidth, keepaspectratio]{images/yoda/neural.png}}   
    \end{subfigure}    
    \hfill  
    \begin{subfigure}[t]{0.159\textwidth}
        \centering
        \frame{\includegraphics[width=\textwidth, keepaspectratio]{images/yoda/seg.png}}   
    \end{subfigure}    
    \hfill  
    \begin{subfigure}[t]{0.159\textwidth}
        \centering
        \frame{\includegraphics[width=\textwidth, keepaspectratio]{images/yoda/both.png}}   
    \end{subfigure}    
    \hfill
    \begin{subfigure}[t]{0.159\textwidth}
        \centering
        \frame{\includegraphics[width=\textwidth, keepaspectratio]{images/yoda/gt.png}}   
    \end{subfigure}
    
    \begin{subfigure}[t]{0.159\textwidth}
        \centering
        \frame{\includegraphics[width=\textwidth, keepaspectratio]{images/yoda_2/baseline.png}}   
        \caption{Gaussian Splatting} 
    \end{subfigure}    
    \hfill  
    \begin{subfigure}[t]{0.159\textwidth}
        \centering
        \frame{\includegraphics[width=\textwidth, keepaspectratio]{images/yoda_2/robust.png}}   
        \caption[]{RobustNeRF} 
    \end{subfigure}    
    \hfill  
    \begin{subfigure}[t]{0.159\textwidth}
        \centering
        \frame{\includegraphics[width=\textwidth, keepaspectratio]{images/yoda_2/neural.png}}   
        \caption[]{+Neural} 
    \end{subfigure}    
    \hfill  
    \begin{subfigure}[t]{0.159\textwidth}
        \centering
        \frame{\includegraphics[width=\textwidth, keepaspectratio]{images/yoda_2/seg.png}}   
        \caption[]{+Segment.} 
    \end{subfigure}    
    \hfill  
    \begin{subfigure}[t]{0.159\textwidth}
        \centering
        \frame{\includegraphics[width=\textwidth, keepaspectratio]{images/yoda_2/both.png}}   
        \caption[]{+Both} 
    \end{subfigure}    
    \hfill
    \begin{subfigure}[t]{0.159\textwidth}
        \centering
        \frame{\includegraphics[width=\textwidth, keepaspectratio]{images/yoda_2/gt.png}}   
        \caption[]{Ground truth} 
    \end{subfigure}    
    \caption{Example comparison of qualitative results for all scenes. We can see that our full version is most effective in ignoring distractors.}
    \label{fig:qual_2}
\end{figure*}
